# Supplementary material for: Autoformalizing Argumentative Material Inferences
Source: arXiv:2609.16991 source file (2026-09-15)
Supplement: Supplementary file 1 [file appendix_setup.tex]

\RequirePackage{amsmath,amssymb}
\RequirePackage{graphicx}
\RequirePackage{booktabs}
\RequirePackage{array}
\RequirePackage{tabularx}
\RequirePackage{enumitem}
\RequirePackage{xcolor}
\RequirePackage{listings}
\RequirePackage{needspace}
\RequirePackage{tcolorbox}
\tcbuselibrary{skins,breakable}


\providecommand{\method}{\textsc{GUARD}}
\providecommand{\vf}{\textsc{Verified-Faithful}}
\providecommand{\rl}{\textsc{Reject-Leaky}}
\providecommand{\amg}{\textsc{Abstain-Missing-Guards}}
\providecommand{\anc}{\textsc{Abstain-Not-Compatible}}
\providecommand{\SoftDiag}{\mathcal{D}}
\providecommand{\Guard}{\mathcal{G}}
\providecommand{\PremAlt}{\mathcal{T}^{-}}
\providecommand{\HypAlt}{\mathcal{H}^{-}}
\newcommand{\appdrop}[1]{{\scriptsize\textcolor{black!55}{$-$#1}}}
\newcommand{\appzero}{\phantom{0}}


\definecolor{appCodeInk}{RGB}{36,47,60}
\definecolor{appCodeKeyword}{RGB}{35,67,99}
\definecolor{appCodeProof}{RGB}{40,88,70}
\definecolor{appCodeComment}{RGB}{102,107,113}
\definecolor{appCodeRule}{RGB}{193,199,205}
\definecolor{appCodeBack}{RGB}{248,249,250}

\lstdefinelanguage{GUARDIsabelle}{
  sensitive=true,
  morekeywords={theory,imports,begin,end,typedecl,consts,
    axiomatization,where,theorem,assumes,shows,using,by,
    proof,qed,from,have,then,show,obtain,fix,let,and},
  morekeywords=[2]{blast,auto,simp,metis,sledgehammer},
  morecomment=[s]{(*}{*)},
  morestring=[b]"
}
\lstdefinestyle{guard-isabelle}{
  language=GUARDIsabelle,
  basicstyle=\footnotesize\ttfamily\color{appCodeInk},
  keywordstyle=\bfseries\color{appCodeKeyword},
  keywordstyle=[2]\bfseries\color{appCodeProof},
  commentstyle=\itshape\color{appCodeComment},
  stringstyle=\color{appCodeInk},
  numbers=left,
  numberstyle=\scriptsize\ttfamily\color{black!45},
  numbersep=5pt,
  stepnumber=1,
  numberblanklines=false,
  firstnumber=1,
  columns=fullflexible,
  keepspaces=true,
  showstringspaces=false,
  showspaces=false,
  showtabs=false,
  tabsize=2,
  breaklines=true,
  breakatwhitespace=true,
  breakautoindent=false,
  breakindent=1em,
  postbreak=\mbox{\textcolor{appCodeComment}{$\hookrightarrow$}\space},
  frame=single,
  framerule=0.35pt,
  framesep=4pt,
  rulecolor=\color{appCodeRule},
  backgroundcolor=\color{appCodeBack},
  xleftmargin=1.8em,
  xrightmargin=0.55em,
  aboveskip=9pt,
  belowskip=10pt,
  captionpos=t,
  abovecaptionskip=5pt,
  belowcaptionskip=7pt,
  literate={∀}{{$\forall$}}1
           {∃}{{$\exists$}}1
           {∧}{{$\wedge$}}1
           {∨}{{$\vee$}}1
           {¬}{{$\neg$}}1
           {⟶}{{$\longrightarrow$}}2
           {⟷}{{$\longleftrightarrow$}}2
           {⇒}{{$\Rightarrow$}}2
           {χ}{{$\chi$}}1
           {’}{{'}}1
}

\lstdefinestyle{guard-isabelle-ascii}{
  style=guard-isabelle,
  literate={ALL}{{$\forall$}}1
           {EX}{{$\exists$}}1
           {<->}{{$\longleftrightarrow$}}2
           {-->}{{$\longrightarrow$}}2
           {=>}{{$\Rightarrow$}}2
           {&}{{$\wedge$}}1
           {|}{{$\vee$}}1
           {~}{{$\neg$}}1
}

\lstdefinestyle{guard-logic}{
  style=guard-isabelle,
  numbers=none,
  xleftmargin=0.55em,
  xrightmargin=0.55em
}

\newenvironment{guardprompt}[2]{%
  \par\refstepcounter{table}\label{#2}%
  \addcontentsline{lot}{table}{\protect\numberline{\thetable}#1}%
  \begin{tcolorbox}[
    enhanced jigsaw,
    breakable,
    colback=black!1.5,
    colframe=black!45,
    colbacktitle=black!6,
    coltitle=black,
    boxrule=0.35pt,
    arc=1pt,
    left=6pt,right=6pt,top=6pt,bottom=6pt,
    fonttitle=\small\bfseries,
    fontupper=\small,
    title={Table~\thetable.\enspace #1},
    title after break={Table~\thetable\ (continued)},
    before skip=7pt,after skip=9pt,
    before upper={\raggedright\setlength{\parindent}{0pt}},
  ]%
}{\end{tcolorbox}\par}


\newcommand{\guarderrorfigure}{%
  \IfFileExists{Figures/autoformalisation_errors.pdf}{%
    \includegraphics[width=0.96\linewidth]{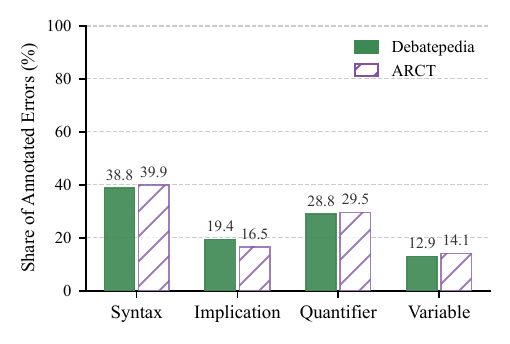}%
  }{%
    \PackageWarning{guard-appendix}{Missing Figures/autoformalisation_errors.pdf}%
    \fbox{\parbox[c][32mm][c]{0.86\linewidth}{\centering\small
      Original figure not included in the supplied files.\par\medskip
      Add \texttt{Figures/}\allowbreak\texttt{autoformalisation\_errors.pdf}
      to the project.}}%
  }%
}
